# Supplementary material for: Perceptual Pat: A Virtual Human System for Iterative Visualization Design
Source: arXiv:2303.06537 source file (2023-03-12)
Supplement: Supplementary file 1 [file 09-appendix.tex]

\appendix

\section{Appendix: Performance of Perceptual Pat Components}
\label{sec:appendix}

Perceptual Pat contains several components based on machine learning models.
Here, we describe the details of each model and report the performance we measure.
We use the pretrained models offered by the original studies.

\subsection{Visual Saliency}
\label{subsec:scanner-deeply}

\paragraph{Scanner Deeply.}

Scanner Deeply~\cite{shin23scannerdeeply} is a \textit{virtual eyetracker for visualization}; it can predict human gaze on a visualization.
Given a data visualization, this framework generates a gaze heatmap using a deep neural network (SimpleNet) trained on over 10k crowdsourced gaze maps for chart images.

\paragraph{Low-Level Salience} 

Low-level Salience is a gaze prediction technique also based on SimpleNet but trained on the Salicon~\cite{jiang15salicon} gaze dataset for natural images drawn from the MS COCO~\cite{lin14coco} dataset.

\paragraph{Performance.}

In Table~\ref{tab:scanner-deeply-tfft}, we show the performance of the Scanner Deeply and Low-level Saliency tested on pairs of gaze heatmaps and visualization images.
We compute six metrics: true-positive (TP), true-negative (TN), false-positive (FP), false-negative (FN), precision, and recall.
To discretize the values of the predicted map, we round the values of each pixel to 0 or 1.
Then, we conduct a pixelwise comparison between the ground-truth model and the predicted heatmap. 
There is not a standard method to evaluate gaze heatmaps, and various existing metrics are devised for specific assumptions and applications. 
For example, Bylinskii et al.~\cite{bylinskii19differentmodels} recommend, on probabilistic prediction maps such as the Scanner Deeply and Low-level Salience, to use Kullback-Leibler divergence for evaluation.
Note that because both the Scanner Deeply and the Low-level salience are probabilistic prediction maps, our method will lower the true positive rates of predicted maps. 
We first show that the performance of the model we use for Low-level Salience is less accurate than the Scanner Deeply for visualization stimulus.
We also observe that Low-level Salience on chart images manifests a large discrepancy between recall and precision.
\revt{That said, it can be a useful source of reference for salience when the visualization is drawn with a natural image as its background or situated within the world, such as for a visualization embedded in Augmented Reality.}

\subsection{Text}
\label{subsec:text-ocr}

We use PyTesseract OCR, a Python version of the Tesseract OCR engine, for the OCR component.
Performance results are given in Table~\ref{tab:yolor-performance}. 
It shows high performance both in terms of precision and recall on a Google Books dataset. 

\subsection{Visual Representation}
\label{subsec:visual-repr}

We employ a object detection model called YoloR~\cite{wang21yolor}; see Table~\ref{tab:yolor-performance} for our performance results.

\begin{table}[htb]
    \centering
    \begin{tabular}{l|cccc|cc}
     
        \toprule
        \rowcolor{gray!10}        
        \textbf{\textsc{Models}} & \textbf{\textsc{TP}} & \textbf{\textsc{TN}} & \textbf{\textsc{FP}} & \textbf{\textsc{FN}} & \textbf{\textsc{Prec.}} & \textbf{\textsc{Rec.}}\\
        \midrule
        A Scanner & 6.31\% & 81.21\% & 10.28\% & 2.20\% &  0.38 & 0.74\\
        Deeply & (1.48) & (8.34) & (1.55) & (0.47) & (0.06) & (0.14)\\
        \rowcolor{gray!10} 
        Low-level  & 5.86\% & 78.49\% & 13.00\% & 2.65\% & 0.31 & 0.69\\
        \rowcolor{gray!10} 
        Salience& (1.21) & (7.34) & (2.24) & (0.51) & (0.04)  & (0.11)\\
        \bottomrule
    \end{tabular}
    \caption{\textbf{Performance of Scanner Deeply and Low-level Salience.}
    We report the performance of those two gaze prediction models tested on the dataset generated by Shin et al.~\cite{shin23scannerdeeply}. 
    This test-set contains 2,712 pairs of gaze heatmaps and charts.
    Prec. and Rec. refer to precision and recall.  }
    \label{tab:scanner-deeply-tfft}
\end{table}

\begin{table}[htb]
    \centering
    \begin{tabular}{l|ccc}
        \toprule
        \rowcolor{gray!10}        
        \textbf{\textsc{Models}} & \textbf{\textsc{Dataset}} & \textbf{\textsc{Prec.}} & \textbf{\textsc{Rec.}}\\
        \midrule
        Tesseract-OCR (OCR) & Google Books & 0.94 & 0.90 \\
        \rowcolor{gray!10} 
        YoloR (Chartjunk) & Microsoft Coco & 0.66 & 0.84\\
        \bottomrule
    \end{tabular}
    \caption{\textbf{Performance of OCR and Chartjunk components.}
    YoloR uses the Microsoft COCO dataset.
    PyTesseract-OCR uses Tesseract-OCR v4.
    These results are drawn from the Tesseract documentation~\cite{PyTesseract_perf} and Wang et al.~\cite{yolor_perf}.}
    \label{tab:yolor-performance}
\end{table}
